# Supplementary material for: View Synthesis of Dynamic Scenes based on Deep 3D Mask Volume
Source: arXiv:2108.13408 source file (2022-11-28)
Supplement: Supplementary file 1 [file supplementary.tex]

% Feel free to add any comments/text here

Suggestions:

%%%%%%%%%%%%%%%%%%%%%%

Abstract, Introduction:
State that we are doing static, binocular video view synthesis
Mention cell phone stereo to do 3D video view synthesis
1. Make use of background to deal with large occlusion
2. Tackle temporal inconsistency

Discuss issues
disocclusion and inaccurate depth estimation
static/dynamic
why adopt 3D mask
why use static cameras
remove loss claims - done

%%%%%%%%%%%%%%%%%%%%%%
Dataset:
Add table for 3.3 - done
3.4 add figure for dataset generation (QR code) - done
Real forward-facing is public or not?

%%%%%%%%%%%%%%%%%%%%%%
Figures:

1. Combine Fig 5 and Fig 7 and move it to p.1 or p.2
Add our result to Fig 7
Show consecutive frames to let people know it's video - done

2. Single-column qualitative results
can be referred to earlier
change to VGG only

3. Pipeline to algorithm part

4. Figure 4 to table - done

5. Figure of lighting changes so that background is bad - supplementary?

%%%%%%%%%%%%%%%%%%%%%%

Algorithm:

1. Add equations - done
median filtering - done

%%%%%%%%%%%%%%%%%%%%%%

Ablations studies:

1. Add discussion - done
VGG mask not interpretable but higher quality - done

2. 2D vs 3D mask ablation studies
move 2D mask results to table 2 - WIP

3. Table 2 STRRED is more obvious, move to 1st column - done

4. selection of other views

5. interpolation instead of extrapolation

6. compare with 3dp?
%%%%%%%%%%%%%%%%%%%%%%
Limitations:
Static and binocular - done

%%%%%%%%%%%%%%%%%%%%%%

Supplementary:

1. videos
2. ablation studies
3. median filter vs. gaussian filter

Todo:
5. View synthesis results from other viewpoints/4 images
7. extreme extrapolation
3. Experiments on interpolation vs extrapolation
(Add to video if results are good)

4. Different kinds of background filtering
6. Examples for failed backgrounds (e.g. lighting changes)

Done:

1. Video showing our results
2. Comparison for different loss functions and effect on masks
